# Supplementary material for: Evaluating Multilingual Text Encoders for Unsupervised Cross-Lingual Retrieval
Source: arXiv:2101.08370 source file (2021-01-21)
Supplement: Supplementary file 1 [file xx-appendix.tex]

\section{Supplementary Material}

\begin{table*}[!t]
\centering

{\scriptsize
{\scriptsize%\fontsize{8pt}{8pt}\selectfont
\begin{tabularx}{\linewidth}{l X X X X X X X X X X}
\toprule
Model & Layer & EN-FI & EN-IT & EN-DE & DE-FI & DE-IT & FI-IT & AVG & w/o FI \\  \midrule
$\text{XLM}_{\text{ISO}}$ & 0 & .004 & .084 & .030 & .004 & .006 & .002 & .022 & .040 \\
& 1 & .016 & .178 & .053 & .006 & .017 & .002 & .045 & .082 \\
& 2 & .011 & .163 & .046 & .006 & .016 & .003 & .041 & .075 \\
& 3 & .007 & .122 & .028 & .007 & .015 & .002 & .030 & .055 \\
& 4 & .005 & .095 & .022 & .006 & .011 & .002 & .023 & .043 \\
& 5 & .003 & .083 & .022 & .004 & .008 & .001 & .020 & .038 \\
& 6 & .002 & .055 & .013 & .003 & .006 & .001 & .013 & .025 \\
& 7 & .002 & .043 & .011 & .004 & .004 & .002 & .011 & .019 \\
& 8 & .002 & .040 & .009 & .004 & .004 & .001 & .010 & .018 \\
& 9 & .002 & .032 & .006 & .003 & .003 & .001 & .008 & .014 \\
& 10 & .001 & .026 & .005 & .001 & .002 & .001 & .006 & .011 \\
& 11 & .001 & .024 & .006 & .002 & .004 & .000 & .006 & .011 \\
& 12 & .001 & .016 & .003 & .001 & .003 & .000 & .004 & .007 \\
& 13 & .001 & .017 & .004 & .001 & .003 & .000 & .004 & .008 \\
& 14 & .001 & .021 & .005 & .001 & .003 & .000 & .005 & .009 \\
& 15 & .001 & .019 & .003 & .001 & .002 & .000 & .004 & .008 \\
& 16 & .001 & .023 & .003 & .001 & .002 & .000 & .005 & .010 \\ \midrule
$\text{mBERT}_{\text{ISO}}$ & 0 & .010 & .141 & .087 & .005 & .017 & .000 & .043 & .082 \\
& 1 & .005 & .116 & .067 & .003 & .015 & .001 & .034 & .066 \\
& 2 & .004 & .085 & .053 & .004 & .013 & .001 & .027 & .050 \\
& 3 & .004 & .075 & .049 & .003 & .014 & .002 & .024 & .046 \\
& 4 & .004 & .081 & .046 & .003 & .014 & .003 & .025 & .047 \\
& 5 & .004 & .088 & .051 & .005 & .022 & .003 & .029 & .054 \\
& 6 & .006 & .091 & .047 & .006 & .031 & .005 & .031 & .056 \\
& 7 & .004 & .074 & .039 & .005 & .027 & .003 & .025 & .047 \\
& 8 & .003 & .070 & .036 & .006 & .020 & .003 & .023 & .042 \\
& 9 & .004 & .061 & .030 & .006 & .021 & .003 & .021 & .037 \\
& 10 & .002 & .032 & .020 & .003 & .016 & .002 & .012 & .023 \\
& 11 & .002 & .040 & .022 & .003 & .017 & .001 & .014 & .026 \\
& 12 & .000 & .027 & .017 & .001 & .005 & .001 & .009 & .016 \\
\bottomrule
\end{tabularx}
}}
\vspace{1mm}
%\caption{Mean Average Precision of fine-tuned models on Europarl (best model of each language-pair is highlighted)}
\label{tab:europarl-paralleldata}
\end{table*}
